# Supplementary material for: On the Economics of Offline Password Cracking
Source: arXiv:2006.05023 source file (2020-06-09)
Supplement: Supplementary file 1 [file AppendixExtraDiscussion.tex]

% !TEX root=zipfs-law.tex

\section{Background on Yahoo! Dataset} \label{apdx:YahooBackground}
In 2012 Yahoo! allowed Bonneau to collect and analyze an anonymized password frequency list based on $N \approx 70$ million user passwords \cite{bonneau2012yahoo}. The data was collected in the form of a list of numbers $f_1 \geq f_2 \geq \ldots$, where $f_1$ (resp. $f_i$) represented the number of users who selected the most common password (resp. $i$'th most common password). Yahoo! initially did not allow Bonneau to publish the frequency corpus he had collected due to potentially unforeseen privacy concerns. Later Yahoo! allowed Blocki et al.~\cite{DPPLists} to release a perturbed version of this dataset using a $\left( \epsilon, \delta \right)$-differential private algorithm~\cite{DPPLists}. 

Differential privacy~\cite{dwork2006calibrating}  provides a strong guarantee of privacy to any individual in a dataset. The general notion is that an adversary will not be able to make any inferences about an individual from this dataset that they would not have been able to make if the individual's data had been excluded. The precise definition is not critical here since we are only interested in understanding how much the frequency corpus was perturbed. We simply observe that smaller values of the parameters $\epsilon$ and $\delta$ imply stronger privacy guarantees, and, consequently, algorithms must add more noise to the data to satisfy this privacy guarantee.  Blocki et al.~\cite{DPPLists} set $\epsilon=0.25, \delta=2^{-100}$ when they perturbed the Yahoo! dataset. Their algorithm ensures that the perturbed list $\tilde{f}= \tilde{f}_1 \geq \tilde{f}_2 \ldots$ remains close to the original frequency list $f = f_1 \geq f_2 \ldots$. In particular, they proved that with high probability $\| f-\tilde{f}\|_1 = O\left(\frac{\sqrt{n}+\ln (1/\delta)}{\epsilon} \right)$, when run on a password frequency list $f$ with $n= f_1+f_2 + \ldots$ users. We refer an interested reader to Bonneau~\cite{bonneau2012yahoo} for more details on how this data was collected and to \cite{DPPLists} for more details on the differentially private algorithm used to perturb the data.

 Formally, let $D$ denote the password dataset, and let $D-\{i\}$ denote the dataset without individual $i$'s password.

 A randomized algorithm $\mathcal{A}$ is said to preserve $\left( \epsilon, \delta \right)$-differential privacy if for any $D$, individual $i$ and any subset $S \subseteq Range\left(\mathcal{A}\right)$ of possible outcomes we have 
	\[\Pr\left[\mathcal{A}(D) \in S \right] \leq e^{\epsilon} \Pr\left[\mathcal{A}\left(D-\{i\}\right) \in S \right] + \delta \ . \]

 $\delta$-approximate implementation of the exponential mechanism~\cite{mcsherry2007mechanism}
 Their algorithm ensures that the perturbed list $\tilde{f}= \tilde{f}_1 \geq \tilde{f}_2 \ldots$ remains close to the original frequency list $f = f_1 \geq f_2 \ldots$. In particular, the proved that $\| f-\tilde{f}\|_1 = O\left(\frac{\sqrt{n}+\ln (1/\delta)}{\epsilon} \right)$, when run on a password frequency list $f$ with $n= f_1+f_2 + \ldots$ users.

 Blocki et al.~\cite{DPPLists} found an efficient $\delta$-approximate implementation of the exponential mechanism~\cite{mcsherry2007mechanism}, which they used to perturb the password frequency list and satisfy $\left( \epsilon, \delta \right)$-differential privacy.

 \section{Fitting the Yahoo! dataset to a PDF-Zipf Distribution} \label{YahooPDF}
 Zipf's law states that the frequency of an element in a distribution is related to its rank in the distribution. In the PDF-Zipf model we expect  $f_i = \frac{C}{i^s}$ users to select the $i'th$ most common password, where $s$ and $C$ are the PDF-Zipf parameters. Normalizing $z = \frac{C}{N}$ by $N$ the number of users we have $p_i = \frac{z}{i^s}$. We can describe these results using a linear equation using logarithms:
$$
\log f_i = \log \frac{C}{i^s} = \log C - s \log i
$$
Now $\log C$ and $-s$ respectively denote intercept and slope of our linear equation. Both parameters can be calculated using the method of least squares, in which case we can calculate the slope
$$
	\hat{ \beta } = -s = \frac{\sum\limits_{i=1}^n \left( x_i - \overline{x}\right)\left( y_i - \overline{y}\right)}{\sum\limits_{i=1}^n \left( x_i - \overline{x}\right)^2}
$$

We used linear least squares regression to fit the Yahoo! dataset using PDF-Zipf's law. We followed the same preprocessng steps used by Wang et al.~\cite{WangZipfLaw14} i.e. we excluded any password that occurs with frequency less than 5~\cite{WangW16}.  Once these have been removed, we examined how well Zipf's law describes the passwords. Our result are shown in table \ref{tab:YahooPDF} and in figure \ref{fig:YahooPDF}.

\begin{table}
\begin{tabular}{| l | c | c | c | c |}

\hline
		&	$s$			& $\log C$ 		& $R^2$			& $z$ \\ \hline
Yahoo!	&	-0.87121 	& 5.99133		& 0.9960		& 0.014 \\ \hline
\end{tabular}\\

\caption{Yahoo! PDF-Zipf}
\label{tab:YahooPDF}
\end{table}

\begin{figure}
\includegraphics[scale=0.3]{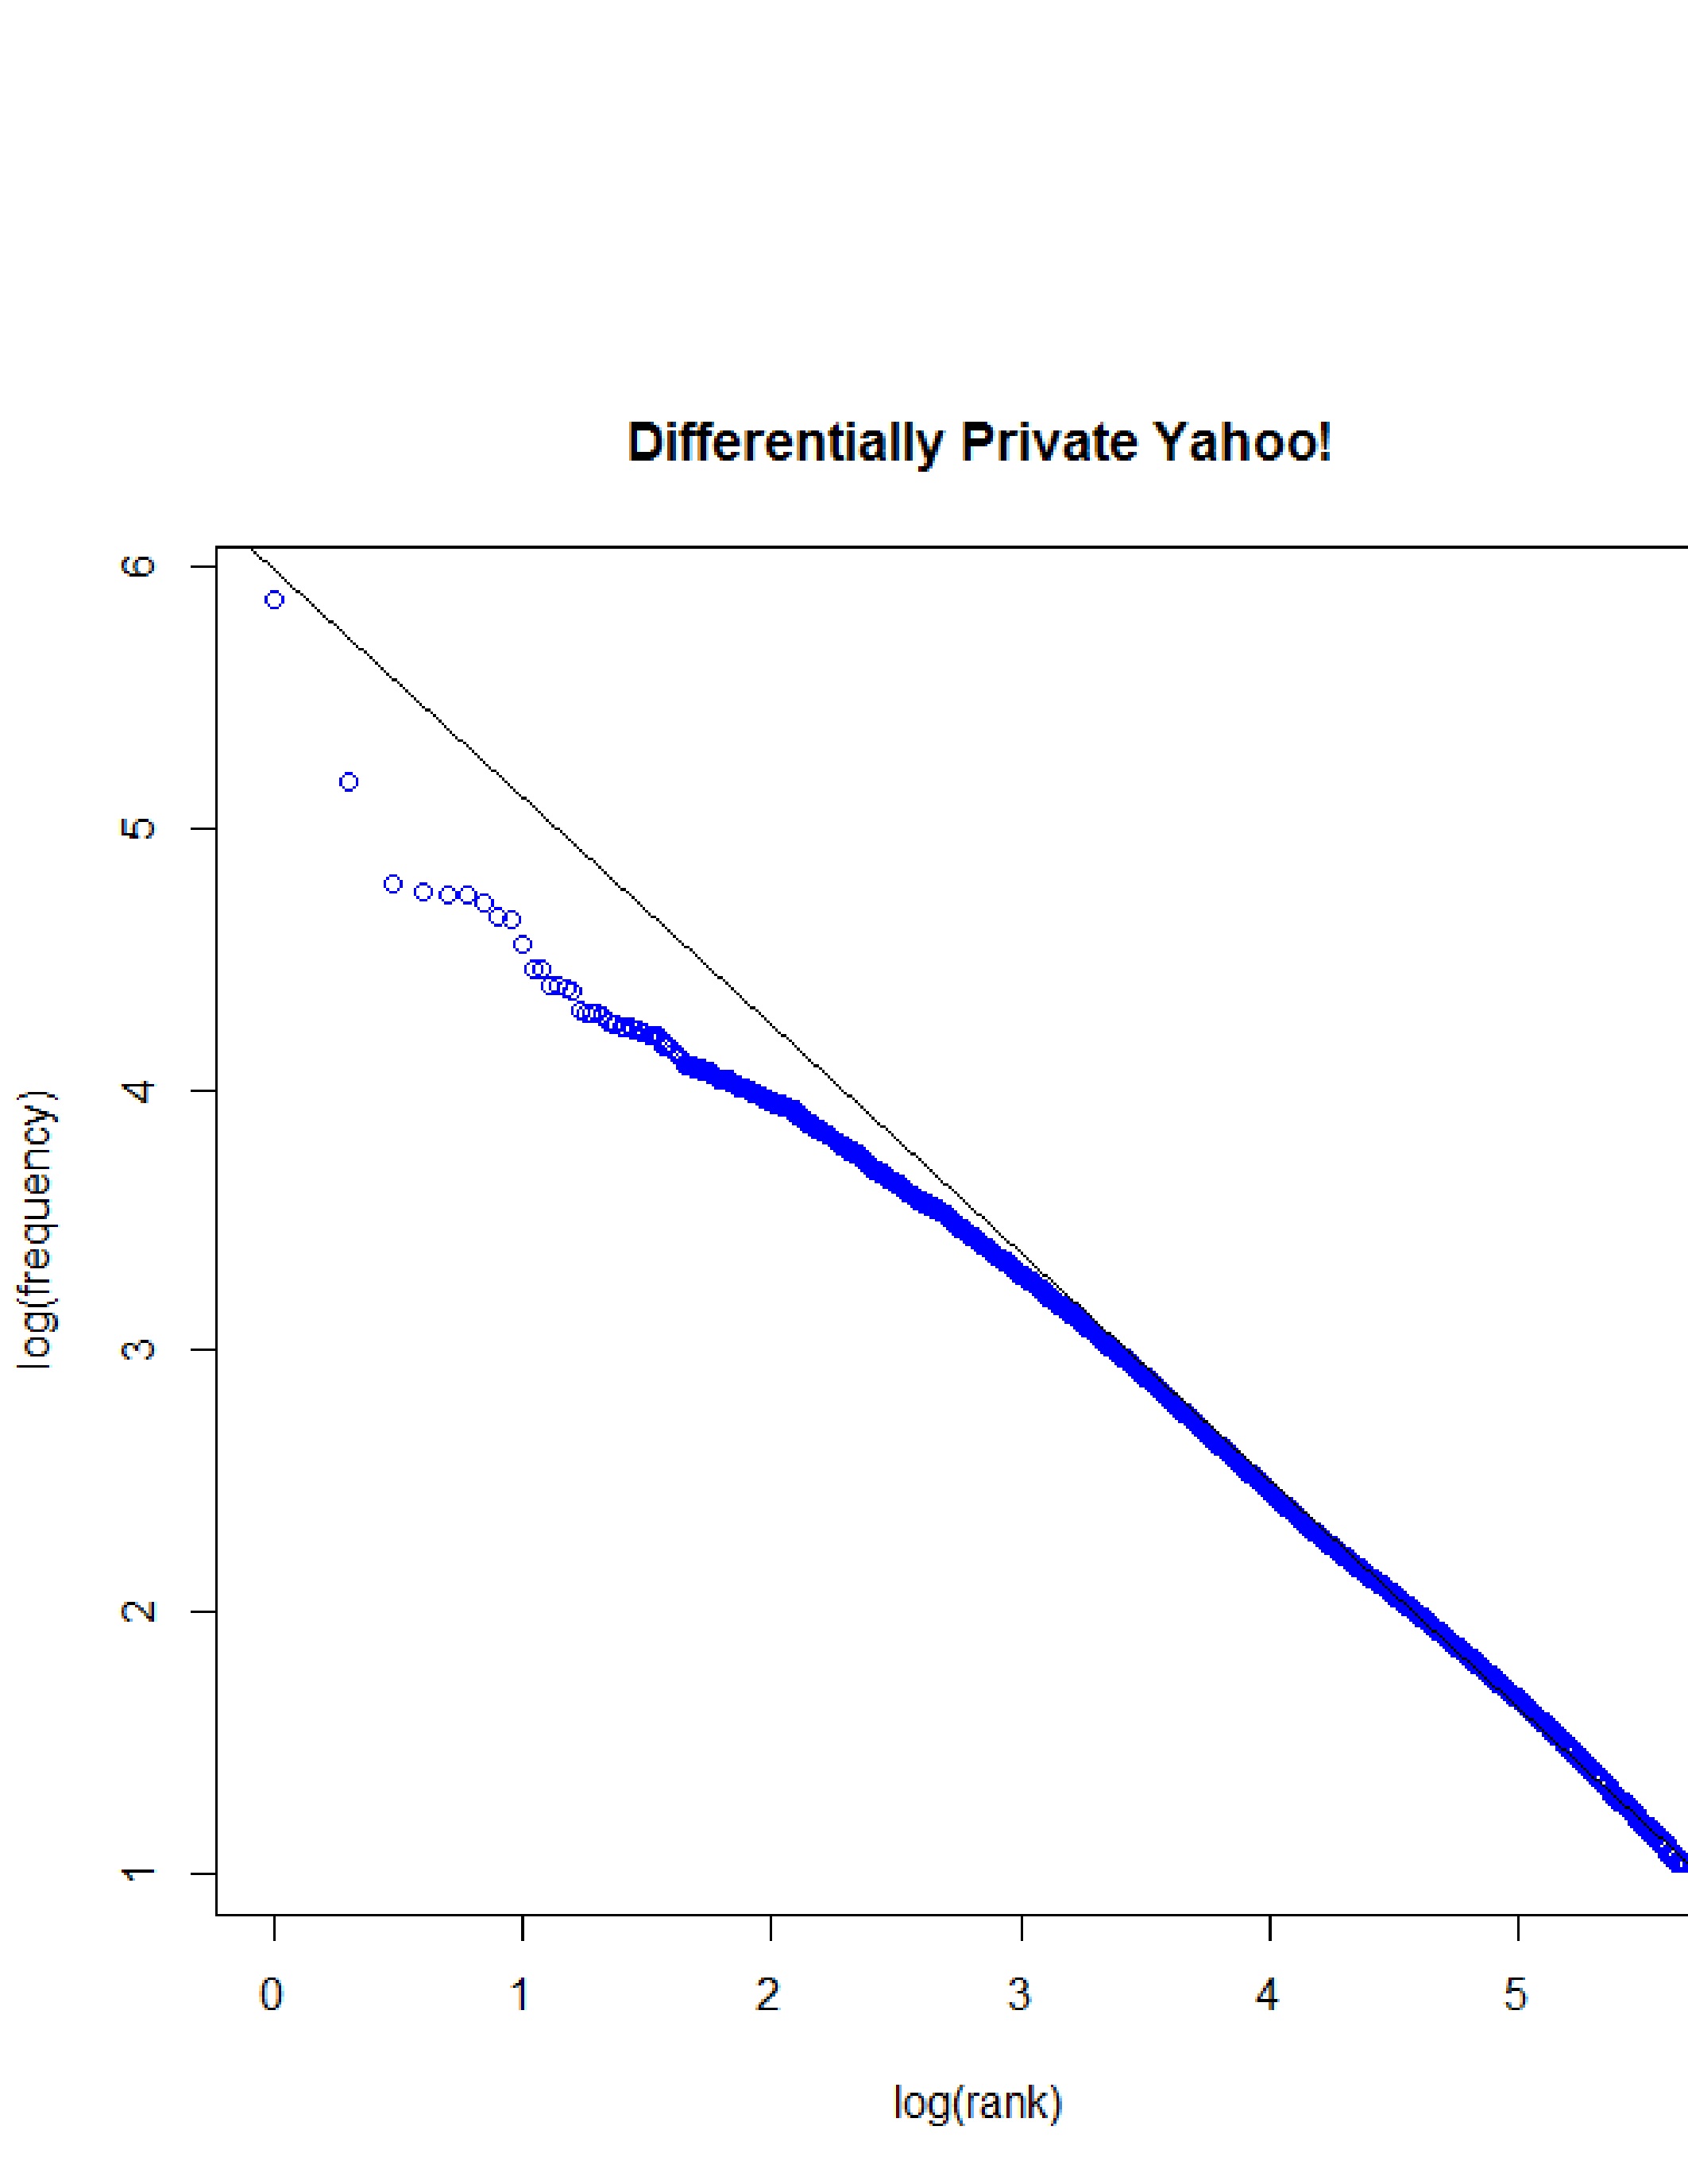}
\centering

\caption{Yahoo! PDF-Zipf}
\label{fig:YahooPDF}
\end{figure}

From these results we conclude that the most common passwords in the Yahoo! dataset are indeed well described by using a Zipf distribution e.g., $R^2 \approx 1$. The parameters obtained by this linear regression are generally consistent with the results Wang et al.~\cite{WangZipfLaw14} reported for other datasets such as RockYou, Tianya, 000webhost, etc\ldots. Furthermore, our experimental results that the differential privacy mechanism does not significantly impact such fittings. The Yahoo! dataset is the largest dataset that has been investigated for a Zipf fitting to this date, and represents the strongest current evidence that real password distributions follow a Zipf distribution.

\subsection{On the Impact of Differential Privacy on PDF-Zipf Fits}  \label{subsec:PDFZipfDP}
The published Yahoo! password frequency lists were perturbed to ensure differential privacy. Before attempting to fit this dataset using Zipf's law we seek to answer the following question: Does this noise, however small, affect our Zipf fitting process in any significant way? We claim that the answer is no, and we offer strong empirical evidence in support of this claim. In particular, we took the RockYou dataset ($N\approx 32.6$ million users) and generated $30$ different perturbed versions of the frequency list by running the $\left( \epsilon, \delta \right)$-differentially private algorithm of Blocki et al.~\cite{DPPLists}. We set $\epsilon=0.25$, the same value that was used to collect the Yahoo! dataset that we analyze. For each of these perturbed frequency lists we compute a PDF-Zipf law fit using the same technique as Wang et al.~\cite{WangZipfLaw14} i.e., excluding passwords that occur with frequency less than $5$ and using linear least squares to compute the PDF-Zipf parameters $s$ and $z$. 

Our results, shown in Table \ref{tab:DPZipLaw}, strongly suggest that the differential privacy mechanism does not impact the parameters $s$ and $z$ in a PDF-Zipf fitting in any significant way. In particular, the parameters $s$ and $z$ we obtain from fitting the original data with a PDF-Zipf model are virtually indistinguishable from the parameters we obtain by fitting on one of the perturbed datasets. Similarly, differential privacy does not affect the fitting's $R^2$ value, a measure of how well the linear regression models the data ($R^2$ values closer to 1 indicate better fittings).  Thus, one can compute Zipf's law parameters for the Yahoo! data collected by \cite{DPPLists} and \cite{bonneau2012yahoo} without worrying about the impact of the $\left( \epsilon, \delta \right)$-differentially private algorithm used to perturb this dataset.

\begin{table}
\begin{tabular}{ | l | c c |}
	\hline
	List Version 			& $s$ 			&  $\sigma_s$		\\ \hline
	RockYou Standard 		& $-0.90790$	& 					\\ \hline
	RockYou Diff. Private 	& $-0.90803$	& $9.35 * 10^{-6}$	\\ \hline
							& $\log C$ 		& $\sigma_{\log C}$ \\ \hline
	RockYou Standard 		& $5.89158$	 	& 					\\ \hline
	RockYou Diff. Private 	& $5.89224$		& $4.99 * 10^{-5}$ 	\\ \hline
							& $R^2$			& $\sigma_{R^2}$	\\ \hline
	RockYou Standard		& $0.99768$		&					\\ \hline
	RockYou Diff. Private	& $0.99771$		& $8.28 * 10^{-7}$	\\ \hline
							& $z$ value		& $\sigma_z$		\\ \hline
	RockYou Standard		& $0.02390$		&					\\ \hline
	RockYou Diff. Private	& $0.02393$		& $2.75 8 10^{-6}$	\\ \hline
% $0.99771$ & $8.28 * 10^{-7}$ &
	 
	 %$.0239$ & $2.74 * 10^{-6}$ \\
%\hline

\end{tabular}

\caption{Impact of Differential Privacy on Zipf's Law Fit}
\label{tab:DPZipLaw}
\end{table}

\subsection{Testing Stability of PDF-Zipf Fit via Subsampling} \label{subsec:PDFZipfStability}
In this section we test the stability of our Zipf's law fit. Bonneau previously investigated the stability of Zipf's law fits for certain specific password statistics such as $\alpha$-guesswork and concluded that the Zipf's law fits for these statistics were not stable~\cite{bonneau2012yahoo}. Wang et al.~\cite{WangZipfLaw14} proposed a new methodology for fitting Zipf parameters i.e., dropping all passwords that occur with frequency less than 5 before fitting Zipf's law to the data. They justified their approach by showing that even if a dataset is generated by sampling from a Zipf's law distribution the tail of this distribution will not follow Zipf's law.  Is this new methodology stable? To investigate, we took several random subsamples from the Yahoo! data and ran the previously described PDF-Zipf fitting procedure. As was done earlier, we eliminate all passwords that occur with frequency less than 5 from the sample that we take from the set as a whole. The results are shown in table \ref{tab:Stability} and figure \ref{fig:Stability}.
\begin{table}
\begin{tabular}{| p{0.7in} | c | c | c | c |}

\hline

Sample Size (Millions)		&	$s$		&	$\log C$	& $R^2$		& $z$ \\ \hline
15							&	0.97658	&	5.00288		& 0.998		& 0.002 \\ \hline
30							&	0.83972	&	5.48908		& 0.997		& 0.004 \\ \hline
45							&	0.86437	&	5.77972		& 0.997		& 0.009 \\ \hline
60							&	0.87794	&	5.96895		& 0.997		& 0.013 \\ \hline
Full						&   0.87121 &	5.99133		& 0.996		& 0.014 \\ \hline

\end{tabular}

\caption{Yahoo! PDF-Zipf with Sub-sampling}
\label{tab:Stability}
\end{table}

\begin{figure}
\includegraphics[scale=0.41]{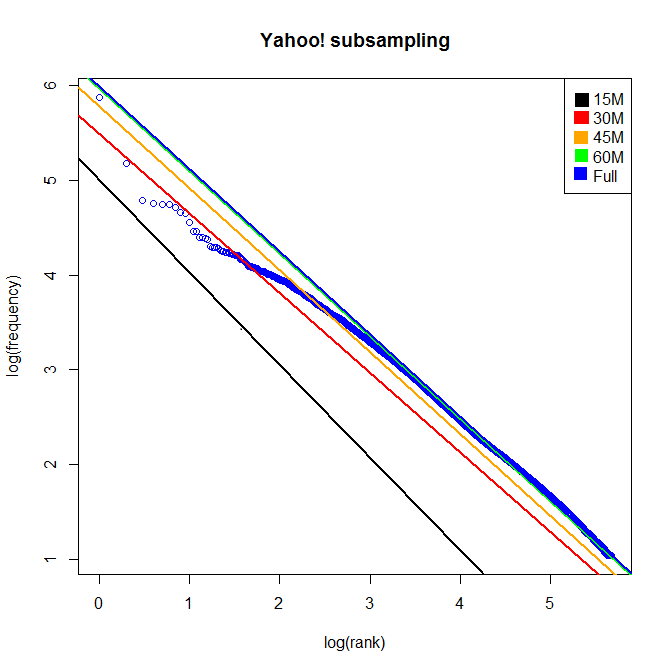}

\caption{Yahoo! PDF-Zipf with Sub-sampling}
\label{fig:Stability}
\end{figure}

We note that the values appear to converge as the sample size increases, to the point where a close inspection of the plotted linear fits will show that it is almost impossible to distinguish between the green (60m subsample) and the blue (full set) regressions. This data seems to suggest that larger subsamples of these Zipfian distributions converge upon the true optimal parameters for the entire dataset.

\section{Extra Plots}
In Figure~\ref{fig:cdf1} the percentage of passwords cracked by a rational adversary compared to possible values of $v/k$ based on the distributions in the two largest datasets, RockYou and Tianya. The RockYou (resp. Tianya) password dataset contained $\approx 32.6$ million (resp. $\approx 30.2$) user passwords in plaintext. The plot shows that as password values increase while hash costs remain constant, the percentage of passwords cracked by a rational adversary increases rapidly. When $v/k > 2.26$ (resp. $v/k > 2.28$) the adversary cracks $100\%$ of RockYou passwords (resp. Tianya).
\begin{figure}[htb]
\centering
\begin{tikzpicture}[scale=0.9] 
\begin{axis}[title style={align=center},
    xlabel={$\log_{10}\left(v/k\right)$},
    ylabel={$\%$ passwords cracked},
		ymin={0},
    ymax={100},
    ylabel shift = -3pt,
    grid=major,
    cycle list = {{red, mark=none}, {blue, mark=none}},
    legend style = {font=\tiny, at={(.05,.95)}, anchor=north west},
    legend entries = {Tianya, RockYou}
  ]
%(1-0.062239*(t-1)^0.155478)/(0.062239*0.155478*t^(0.155478-1)) at t=1000
%log(2*10^7)/log(10)
%0.037433*(10^7)^0.187227
\addplot coordinates{(2.012, 6.22) (2.819, 8.9) (3.64424, 12.73) (4.46, 18.2178) (5.26, 26.06) (6.034, 37.278) (6.75, 53.325) (7.3, 76.2796) (7.3576, 100)};
\addplot coordinates{(2.012, 3.74) (2.819, 5.76) (3.64424, 8.8656) (4.46, 13.6438) (5.26, 20.9973) (6.034, 32.3139) (6.75, 49.7298) (7.3, 76.5321) (7.354, 100)}; 
\end{axis} 
\end{tikzpicture}
\caption{$\%$ passwords cracked by a rational adversary for various values of $v/k$.}\label{fig:cdf1}
\end{figure}
