# Supplementary material for: On the Economics of Offline Password Cracking
Source: arXiv:2006.05023 source file (2020-06-09)
Supplement: Supplementary file 3 [file appendix.tex]

% !TEX root=sp-main.tex
The appendix is divided into three sections. In Section \ref{apdx:PDFZipfLawAnalysis} derives a finite threshold that characterizes the behavior of a rational adversary when passwords follow PDF-Zipf's law.

\section{PDF Zipf's law} \label{apdx:PDFZipfLawAnalysis}
Previously in section \ref{sec:ZipfLawAnalysis} we showed that there is a finite threshold $T(y,r)$ which characterizes the behavior of a rational adversary when passwords follow a CDF-Zipf's law with parameters $y$ and $r$ i.e., $\lambda_i = yi^r$. We now extend our analysis to PDF-Zipf's law. Recall that PDF-
Zipf's Law states that there exist constants $0<s<1$ and $z$, such that $p_n=\frac{z}{n^s}$, where $p_n$ is the probability of the $n$\th ranked password. Also recall that $v$ is the value of obtaining a password, and $k$ is the cost per password attempt. We show that  for $\frac{v}{k}\ge \max_t(\frac{t^s}{z}-\frac{t}{1-s})$ a rational adversary continues until all passwords are cracked. 

 Suppose an adversary continuously guesses passwords until either the password is cracked or some threshold $t$ guesses have been made. For an integer $t>0$, the expected revenue $R$ of trying the $t$ most frequent passwords is 
\[R(t)=v\left(\sum_{n=1}^t p_n\right)\]
and the expected cost $C$ is
\[C(t)=k\left(t\left(1-\sum_{n=1}^t p_n\right)+\sum_{n=1}^t np_n\right).\]

Applying PDF-Zipf's Law we have
\[
\sum_{n=1}^t p_n=\frac{z}{1^s}+\frac{z}{2^s}+\ldots+\frac{z}{t^s}\approx\int_0^t\frac{z}{x^s}\,dx=\frac{zt^{1-s}}{1-s}.
\]
Similarly,
\begin{align*}
\sum_{n=1}^t np_n&=\frac{z}{1^{s-1}}+\frac{z}{2^{s-1}}+\ldots+\frac{z}{t^{s-1}}\\
&\approx\int_0^t\frac{z}{x^{s-1}}\,dx=\frac{zt^{2-s}}{2-s}.
\end{align*}
Hence, we approximate the expected revenue with the function
\[R(t)\approx\frac{vzt^{1-s}}{1-s}\]
and the expected cost with the function
\[C(t)\approx k\left(t\left(1-\frac{zt^{1-s}}{1-s}\right)+\frac{zt^{2-s}}{2-s}\right).\]
Then the marginal revenue is
\[\frac{dR}{dt}=vzt^{-s}=\frac{vz}{t^s}\]
and the marginal cost is
\[\frac{dC}{dt}=k\left(1-\left(\frac{2-s}{1-s}\right)zt^{1-s}+zt^{1-s}\right).\]

A rational adversary can be assumed to pick an optimal threshold which maximizes the utility. 
Therefore, $\frac{dR}{dt}(t)=\frac{dC}{dt}(t)$ so that
\begin{align*}
\frac{vz}{t^s}&=k\left(1-\left(\frac{2-s}{1-s}\right)zt^{1-s}+zt^{1-s}\right)\\
\frac{v}{k}&=\frac{t^s}{z}\left(1-\left(\frac{2-s}{1-s}\right)zt^{1-s}+zt^{1-s}\right)\\
&=\frac{t^s}{z}-\left(\frac{2-s}{1-s}\right)t+t\\
&=\frac{t^s}{z}-\frac{t}{1-s}.
\end{align*}
Since $0<s<1$, we have
\[\frac{v}{k}=\frac{t^s}{z}-\frac{t}{1-s}<\frac{t}{z}-\frac{t}{1-s}.\]
On the other hand,
\[\frac{v}{k}=\frac{t^s}{z}-\frac{t}{1-s}>\frac{t^s}{z}-\frac{t^s}{1-s}.\]
Thus, the rational adversary will choose some optimal threshold $\frac{vz(1-s)}{k(1-s-z)}<T<\left(\frac{vz(1-s)}{k(1-s-z)}\right)^{1/s}$. 
Hence, at least $\sum_{n=1}^Tp_n$ passwords will be compromised. 
From Zipf's Law, we have
\begin{align*}
\sum_{n=1}^Tp_n&=\sum_{n=1}^T\frac{z}{n^s}\\
&>\int_1^{T+1}\frac{z}{x^s}\,dx=\frac{z(T+1)^{1-s}}{1-s}-\frac{z}{1-s}.
\end{align*}
Therefore, at least $\frac{z\left(\frac{vz(1-s)}{k(1-s-z)}+1\right)^{1-s}}{1-s}-\frac{z}{1-s}$ fraction of passwords will be compromised.
On the other hand, 
\begin{align*}
\sum_{n=1}^Tp_n&=\sum_{n=1}^T\frac{z}{n^s}\\
&<\int_0^{T}\frac{z}{x^s}\,dx=\frac{z(T)^{1-s}}{1-s}.
\end{align*}
Therefore, at most $\frac{z\left(\frac{vz(1-s)}{k(1-s-z)}\right)^{(1-s)/s}}{1-s}$ fraction of passwords will be compromised.

Moreover, note that for $\frac{v}{k}\ge\max_t(\frac{t^s}{z}-\frac{t}{1-s})$, the marginal utility for the adversary is always positive, and so a rational adversary continues until all passwords are cracked. Note that for $f(t)=\frac{t^s}{z}-\frac{t}{1-s}$, we have $f'(t)=\frac{st^{s-1}}{z}-\frac{1}{1-s}$ and $f''(t)=\frac{s(s-1)t^{s-2}}{z}<0$ for all $0<s<1$ and $t>0$. 
Hence, the maximum of $f$ occurs at $f'(t)=0$, or equivalently, $t=\left(\frac{z}{s(1-s)}\right)^{\frac{1}{s-1}}$.
Thus, for
\[\frac{v}{k}\ge\frac{\left(\frac{z}{s(1-s)}\right)^{\frac{s}{s-1}}}{z}-\frac{\left(\frac{z}{s(1-s)}\right)^{\frac{1}{s-1}}}{1-s},\]
a rational adversary will crack all passwords.

\subsection{Analysis with PDF-Zipf's law}

The data collected by \cite{WangW16} from the Tianya forums conforms to $z=0.018684$ and $s=0.895411$. Thus,
%We have the following data points for $(v/k, t, T, \sum_{n=1}^Tp_n)$:
%$(10, 0.18408, 0, 0)$
%$(25, 0.524084, 0, 0)$
%$(50, 1.15899, 1, 0.018684)$
%$(100, 2.56858, 2, 0.028728)$
%$(250, 7.38288, 7, 0.052564)$
%$(500, 16.4646, 16, 0.071510)$
%$(1000, 36.843, 36, 0.092245)$
%$(2500, 107.513, 107, 0.123371)$
%$(5000, 243.081, 243, 0.149384)$
%$(10000, 552.852, 552, 0.177781)$
%$(25000, 1656.78, 1656, 0.219860)$
%$(50000, 3842.16, 3842, 0.255540)$
%$(100000, 9020.62, 9020, 0.295081)$
%$(250000, 28611.8, 28611, 0.354503)$
%$(500000, 70520.7, 70520, 0.406201)$
%$(1000000, 180908, 180908, 0.465659)$
%$(2500000, 711327, 711327, 0.563216)$
%$(5000000, 2883750, 2883750, 0.678494)$
%END
%$(10, 0.227477, 0.003871)$
%$(25, 0.568692, 0.008614)$
%$(50, 1.13738, 0.014771)$
%$(100, 2.27477, 0.023597)$
%$(250, 5.68692, 0.039276)$
%$(500, 11.3738, 0.053764)$
%$(1000, 22.7477, 0.0701627)$
%$(2500, 56.8692, 0.094455)$
%$(5000, 113.738, 0.114722)$
%$(10000, 227.477, 0.136635)$
%$(25000, 568.692, 0.168429)$
%$(50000, 1137.38, 0.194297)$
%$(100000, 2274.77, 0.222319)$
%$(250000, 5686.92, 0.262634)$
%$(500000, 11373.8, 0.295808)$
%$(1000000, 22747.7, 0.331479)$
%$(2500000, 56869.2, 0.382734)$
%$(5000000, 113738, 0.424996)$
%http://www.wolframalpha.com/input/?i=evaluate(x*(y*x*(1-z)%2F(1-z-x))%5E((1-z)%2Fz)%2F(1-z),+x%3D0.018684,+y%3D100000,+z%3D0.895411)
%evaluate(y*(r*y*v/(r-r*y-y))^r, y=.062239, v=1000000, r=.155478)
\begin{figure}[htb]
\centering
\begin{tikzpicture}[scale=0.9] 
\begin{axis}[title style={align=center},
    xlabel={$\log_{10}\left(v/k\right)$},
    ylabel={Fraction of passwords cracked},
    ymax={1},
    ylabel shift = -3pt,
    grid=major,
    %small,
    cycle list = {{red, mark=none},  {blue, mark=none}, {green, mark=none}},
    legend style = {font=\tiny, at={(.05,.95)}, anchor=north west},
    legend entries = {actual, lower bound, upper bound}
  ] 
\addplot coordinates{ (1, 0) (1.4, 0) (1.7, 0.018684) (2, 0.028728) (2.4, 0.052564) (2.7, 0.071510) (3, 0.092245) (3.4, 0.123371) (3.7, 0.149384) (4, 0.177781)
				(4.4, 0.219860) (4.7, 0.255540) (5, 0.295081) (5.4, 0.354503) (5.7, 0.406201) (6, 0.465659) (6.4, 0.563216) (6.7, 0.678494)}; %(6.741211, 1)
\addplot coordinates{ (1, 0.003871) (1.4, 0.008614) (1.7, 0.014771) (2, 0.023597) (2.4, 0.039276) (2.7, 0.053764) (3, 0.0701627) (3.4, 0.094455) (3.7, 0.114722) 
				(4, 0.136635) (4.4, 0.168429) (4.7, 0.194297) (5, 0.222319) (5.4, 0.262634) (5.7, 0.295808) (6, 0.331479) (6.4, 0.382734) (6.7, 0.424996)};
\addplot coordinates{ (1, 0.150269) (1.4, 0.167245) (1.7, 0.181349) (2, 0.196642) (2.4, 0.218856) (2.7, 0.237312) (3, 0.257325) (3.4, 0.286394) (3.7, 0.310546) 
				(4, 0.336734) (4.4, 0.374774) (4.7, 0.406379) (5, 0.440649) (5.4, 0.490427) (5.7, 0.531785) (6, 0.576632) (6.4, 0.641771) (6.7, 0.695892)}; %(7, 0.754578)
\end{axis} 
\end{tikzpicture}
\caption{Passwords cracked by a rational adversary for various values of $v/k$.}\label{fig:tianya}
\end{figure}

For the datasets provided by \cite{WangW16}, we can analyze the minimum threshold $v/k$ for which an economic adversary chooses to crack all passwords.
%evaluate((z/(s(1-s)))^(s/(s-1))/z - ( z / (s(1-s)))^(1/(s-1))/(1-s), z=0.025464, s=0.913760)
\[\begin{tabular}{|c|cc|c|}\hline
Dataset & $z$ & $s$ & $v/k$ Threshold \\\hline
RockYou & $0.025464$ & $0.913760$ & $5.34698\times10^5$ \\\hline
000webhost & $0.000512$ & $0.603784$ & $9.05139\times10^6$ \\\hline
Battlefield & $0.003522$ & $0.692898$ & $9.10408\times10^5$ \\\hline
Tianya & $0.018684$ & $0.895411$ & $5.51075\times10^6$ \\\hline
Dodonew & $0.002566$ & $0.740560$ & $2.26466\times10^7$ \\\hline
CSDN & $0.008176$ & $0.853028$ & $1.36857\times10^8$ \\\hline
Mail.ru & $0.006142$ & $0.768912$ & $2.74082\times10^6$ \\\hline
Gmail & $0.007013$ & $0.793667$ & $5.39374\times10^6$ \\\hline
Flirtlife.de & $0.016824$ & $0.745634$ & $1.8342\times10^4$ \\\hline
\textcolor{blue}{Yahoo!} & \textcolor{blue}{$0.01413$} & \textcolor{blue}{$0.871$} & \textcolor{blue}{$1.09733\times10^7$} \\\hline
\end{tabular}\]

\jnote{Ben's results indicate that (1) the differentially private Yahoo! dataset does fit Zipf's law (PDF) if you omit infrequent passwords, (2) the parameters are pretty similar for Yahoo! and RockYou, and (3) differential privacy doesn't seem to alter the Zipf's law fit in any significant way (in particular, if you perturb the RockYou dataset to satisfy differential privacy and then run linear regression your slope, y-intercept and $R^2$ value are still pretty similar. } 

\jnote{For Yahoo!, fitting PDF Zipf to the differentially private dataset, we have $f_i = \frac{C}{r^s}$ for $C= 10^{5.991}\approx 979,490$ and $s=0.871$. Alternatively, $p_i = \frac{z}{i^s}$ for $z=C/N \approx 0.01413$ --- here $N = \#$users in the sanitized Yahoo! dataset.}

Alternatively, if we define $\tau$ as the number of time steps in performing a hash, we can examine the relationship between $v/k$ and $\log_2(\tau)$ at the threshold for which an economic adversary chooses to crack all passwords. 
Specifically, if we consider any hash function which is achieved via key stretching, then $\tau$ is also the number of iterations performed by the hash function.
%\begin{figure}[H]
%\centering
%\begin{tikzpicture}[scale=1] 
%\begin{axis}[title style={align=center},
   %xlabel={$k$},
   %ylabel={$V$},
   %ylabel shift = -3pt,
	 %%xmin={0},
	 %%xmax={12},
   %grid=major,
   %legend style = {font=\tiny, at={(.95,.05)}, anchor=south east},
	 %legend entries = {RockYou, 000webhost, Tianya, Dodonew}
   %%legend entries = {RockYou, 000webhost, Battlefield, Tianya, Dodonew, CSDN, Mail.ru, Gmail, Flirtlife.de}
  %] 
%
%\addplot{5.34698*x*10^5};
%\addplot{9.05139*x*10^6};
%%\addplot{9.10408*x*10^5};
%\addplot{5.51075*x*10^6};
%\addplot{2.26466*x*10^7};
%%\addplot{1.36857*x*10^8};
%%\addplot{2.74082*x*10^6};
%%\addplot{5.39374*x*10^6};
%%\addplot{1.8342*x*10^4};
%\end{axis} 
%\end{tikzpicture}
%\caption{Necessary $k$ to avoid all passwords cracked by an economic adversary.} \label{fig:vk1}
%\end{figure}

\begin{figure}[htb]
\centering
\begin{tikzpicture}[scale=0.9] 
\begin{axis}[title style={align=center},
	 title={Minimum $v/k$ at which all passwords are cracked},
   xlabel={$\log_2(\tau)$},
   ylabel={$v/k (\times10^{16})$},
	 xmin={7},
	 xmax={35},
	 ymin={0},
	 ymax={1},
   ylabel shift = -3pt,
   grid=major,
	 cycle list = {{red, mark=none},  {orange, mark=none}, {purple, mark=none}},
   legend style = {font=\tiny, at={(.05,.95)}, anchor=north west},
	 legend entries = {RockYou, Yahoo!, Tianya, Dodonew, $v^\$=\$4$ (estimate),$v^\$=\$30$ (estimate), Dropbox $\tau$, AshleyMadison $\tau$, LastPasss $\tau$}
  ] 

\addplot[color=black, domain=7:35]{5.34698*10^5*(2^x)/10^16};
\addplot[color=green, domain=7:30]{1.09733*10^7*(2^x)/10^16};
%\addplot{9.10408*10^5*exp(ln(2)*x)};
\addplot[color=red, domain=7:35]{5.51075*10^6*(2^x)/10^16};
\addplot[color=blue, domain=7:30]{2.26466*10^7*(2^x)/10^16};
\addplot[style=dotted, domain=7:35]{0.057143};
\addplot[style=dashed, domain=7:35]{0.057143*30.0/4.0};
\addplot[mark=x] coordinates{ (8, 0)  (8,0.25) (8,0.5) (8,0.75) (8, 50)};
\addplot[mark=triangle] coordinates{ (12, 0)(12,0.25)  (12,0.5) (12,0.75) (12, 50)};
\addplot[mark=square] coordinates{ (16.66667, 0) (16.66667,0.25) (16.66667,0.5) (16.66667,0.75) (16.66667, 50)};
%\addplot{1.36857*10^8*exp(ln(2)*x)};
%\addplot{2.74082*10^6*exp(ln(2)*x)};
%\addplot{5.39374*10^6*exp(ln(2)*x)};
%\addplot{1.8342*10^4*exp(ln(2)*x)};
\end{axis} 
\end{tikzpicture}
\caption{$\tau$ is number of hash iterations, while $v/k$ is the ratio of the value of a password to the cost of a single hash iteration. The dashed line represents an estimate for SHA-256 for passwords valued at $\$4$. The vertical lines represent the number of iterations for Dropbox, AshleyMadison, LastPass, from left to right.} \label{fig:zipf:data}
\end{figure}

Looking to monetary values of $v$ and $k$, we respectively define $v^{\$}$ and $k^{\$}$, in dollars, as the value of a password and the cost of computing a hash function (multiple times if necessary).  
\cite{BonneauS14} observes that in 2013, Bitcoin miners were able to perform approximately $2^{75}$ SHA-256 hashes in exchange for bitcoin rewards worth about $\$257M$. 
Correspondingly, one can estimate the cost of evaluating a SHA-256 hash to be approximately $C_H=\$7\times10^{-15}$. 
\snote{Find source for monetary estimates of passwords}
\bnote{Bonneau provides an estimate in "Towards reliable storage of 56 bit secrets in human memory" paper. It doesnt seem to match this though, he claims it is closer to $8.5 \times 10^{-16}$} \jnote{  Bonneau was trying to argue that 56 bit secrets are sufficient. Thus, he conservatively assumed that a government agency like NSA might be able to reduce the cost of computing SHA256 by an additional factor of $8$--- note that $8\times 8.5 \times 10^{-16}  \approx 7 \times 10^{-15}$. We are trying to argue that an economically motivated adversary will crack all passwords so I think it makes sense to stick with the original estimate $C_H=\$7\times10^{-15}$. }
Estimating that the value of a password may range from $\$4$ and $\$30$, Figure~\ref{fig:necessary:iterations} shows the necessary number of hash iterations to avoid an economic adversary finding all passwords.

\begin{figure}[htb]
\centering
\begin{tikzpicture}[scale=0.9] 
\begin{axis}[title style={align=center},
  xlabel={$\log_2(\tau)$},
  ylabel={$v$},
	xmin={0},
	xmax={30},
	ymin={0},
	ymax={50},
  ylabel shift = -3pt,
  grid=major,
  legend style = {font=\tiny, at={(.05,.95)}, anchor=north west},
	legend entries = {Dodonew, Yahoo!, $v^{\$}=\$4$ (estimate), $v^{\$}=\$30$ (estimate),$\max \#$ SHA256 hashes in 1sec $(10^7)$, Dropbox $\tau$, AshleyMadison $\tau$, LastPasss $\tau$}
  ] 
\addplot[color=blue, domain=0:30]{(2.26466*10^7)*(7*10^-15)*(2^x)};
\addplot[color=green, domain=0:30]{(1.09733*10^7)*(7*10^-15)*(2^x)};
\addplot[color=black, style=dotted, domain=0:30]{4};
\addplot[color=black, style=dashed, domain=0:30]{30};
\addplot[color=red,mark=diamond] coordinates {(23.2635,0) (23.2635,20) (23.2635,40) (23.2635,50)};
\addplot[mark=x] coordinates{ (8, 0)  (8,20) (8,40) (8, 50)};
\addplot[mark=triangle] coordinates{ (12, 0)(12,20)  (12,40) (12, 50)};
\addplot[mark=square] coordinates{ (16.66667, 0) (16.66667,20) (16.66667,40)  (16.66667, 50)};
\addplot[mark=*] coordinates {(24.5888,4)};
\addplot[mark=*] coordinates {(27.4957,30)};
\addplot[mark=*] coordinates {(25.6341,4)};
\addplot[mark=*] coordinates {(28.541,30)};
\end{axis} 
\end{tikzpicture}
\caption{For $v^{\$}=\$4$, we need at least $2^{24.5888}$ hash iterations and for $v^{\$}=\$30$, we need at least $2^{27.4957}$ hash iterations simply for the adversary to not break \emph{all} passwords for Dodonew or Yahoo!. However, more than $2^{23.2635}$ hash iterations represent an intolerable delay for the authentication server.}
\label{fig:necessary:iterations}
\end{figure}

Moreover, for known breaches, the cryptographic functions used are known. 
For example, AshleyMadison used BCRYPT with a cost factor of $12$, which corresponds to $\tau=2^{12}$ hash iterations. 
Dropbox used BCRYPT with a cost factor of $8$. 
LastPass used PBKDF2-SHA256 with $10^5$ rounds of hashing on their server, and an additional $5000$ rounds on the client before the master password is sent to the server.
%We further assume that Yahoo! uses BCRYPT with level $14$.
If we again assume $k^{\$}=\$7\times10^{-15}$, then using $k^{\$}=\tau C_H$, we examine the security of these companies with respect to various thresholds in Figure~\ref{fig:v:threshold2}.
%Since $k^{\$}=\$1*2^{-24}$ for Dropbox, then we deduce that for BCRYPT, $C_H=\$1*2^{-16}$.
\snote{This is all done assuming BRCYPT hash iteration costs $\$7*10^{-15}$.} \jnote{A few citations in support. A VLSI implementation of the blowfish encryption/decryption
algorithm \url{http://dl.acm.org/citation.cfm?id=368449}. Iteration Bound Analysis and Throughput
Optimum Architecture of SHA-256 (384,512) for
Hardware Implementations \url{https://securewww.esat.kuleuven.be/cosic/publications/article-958.pdf}. SCRYPT \url{https://www.tarsnap.com/scrypt/scrypt.pdf}. \url{http://www.heliontech.com/downloads/fast_hash_asic_datasheet.pdf}  or An ASIC implementation of low power and high throughput
blowfish crypto algorithm \url{http://ac.els-cdn.com/S0026269210000595/1-s2.0-S0026269210000595-main.pdf?_tid=2bb31a9a-a55c-11e6-a451-00000aacb35d&acdnat=1478572777_5793099320ebaaa30aa95e201e3ffd5b} }
\jnote{Apparently, half of Dropbox users were protected by SHA1 (some upgrade issue maybe?). See \url{https://www.troyhunt.com/the-dropbox-hack-is-real/}. LastPass used PBKDF2-SHA256 with $10^5$ rounds of hashing on their server, and an additional $5,000$ rounds on the client before the master password is sent to the server. Yahoo! is unknown right now, but based on the fact that the authentication delay is short I am fairly confident that they run BCRYPT with level $\leq 14$ at most. }

\begin{figure}[htb]
\centering
\begin{tikzpicture}[scale=0.9] 
\begin{axis}[title style={align=center},
   xlabel={$\log_{10}($Threshold$)$},
   ylabel={$v^{\$}$},
	 xmin={5},
	 xmax={12},
	 ymin={0},
	 ymax={50},
	 %extra x ticks = {7.04034, 6.741211, 5.728109, 7.35503},
	 %extra x tick labels = {},
	 %extra x tick style = {major grid style=red, tick align=outside, tick style=red},
   ylabel shift = -3pt,
   grid=major,
	 cycle list = {{red, mark=none},  {orange, mark=none}, {yellow, mark=none}, {purple, mark=none}},
	 legend style = {font=\tiny, at={(.05,.95)}, anchor=north west},
	 legend entries = {AshleyMadison, Dropbox, LastPass, $v^{\$}=\$4$, $v^{\$}=\$30$, RockYou, Tianya, Yahoo!, Dodonew}
  ] 
\addplot[color=green, domain=5:12]{(10^x)*(7*10^-15)*(2^12)};
\addplot[color=blue, domain=5:12]{(10^x)*(7*10^-15)*(2^8)};
\addplot[color=black, domain=5:11]{(10^x)*(7*10^-15)*(5000+10^5)};
\addplot[color=black, style=dotted, domain=5:12]{4};
\addplot[color=black, style=dashed, domain=5:12]{30};

\addplot[mark=x] coordinates{ (5.728109, 0) (5.728109, 10) (5.728109, 50)};
\addplot[mark=*] coordinates{ (6.741211, 0) (6.741211, 10) (6.741211, 50)};
\addplot[mark=triangle] coordinates{ (7.04034, 0) (7.04034, 10)  (7.04034, 50)};
\addplot[mark=square] coordinates{ (7.35503, 0) (7.35503, 10) (7.35503, 50)};

\end{axis} 
\end{tikzpicture}
\caption{$v^{\$}$ versus thresholds for various companies. The vertical lines represent the thresholds for RockYou, Tianya, Yahoo!, Dodonew, from left to right.}
\label{fig:v:threshold2}
\end{figure}

On the other hand, the cost of computing memory hard functions, such as SCRYPT, may not scale linearly with the number of time steps. In fact, recent results of Alwen et al.~\cite{ACPRT17} suggest that SCRYPT is indeed maximally memory hard $k\approx \tau^2$. \footnote{For data-independent memory hard functions the picture is less clear. Alwen and Blocki~\cite{C:AlwBlo16} recently gave attacks on data-independent memory hard functions including Argon2i, winner of the Password Hashing Competition~\cite{PHC}. However, Alwen et al.~\cite{ABP16} construct a family of data-independent memory hard functions with computational complexity $\tilde{\Omega}(n^2)$, where $n$ is the number of nodes in the graph.} Hence, for memory hard functions, we take $k^{\$}=\tau C_H+\tau^2 C_{mem}$, where $C_{mem}$ is the cost of maintaining a hash value in memory. 

If we take $C_{mem}=\frac{C_H}{3000}$, the difference is in Figure~\ref{fig:mhf}.

\begin{figure}[htb]
\centering
\begin{tikzpicture}[scale=0.9] 
\begin{axis}[title style={align=center},
	 title={Effects of Memory Hard Functions},
   xlabel={$\log_2(\tau)$},
   ylabel={$v^{\$}$},
	 xmin={14},
	 xmax={30},
	 ymin={0},
	 ymax={35},
   ylabel shift = -3pt,
   grid=major,
   legend style = {font=\tiny, at={(.05,.95)}, anchor=north west},
	 legend entries = {RockYou, Tianya, Yahoo!, RockYou MHF, Tianya MHF, Yahoo! MHF,$(\tau=10^7)$,  LastPasss $\tau$, $v^{\$}=\$4$ (estimate), $v^{\$}=\$30$ (estimate)}
  ] 

\addplot[color=black, domain=14:30]{(5.34698*10^5)*7*(10^-15)*(2^x)};
\addplot[color=red, domain=14:30]{(5.51075*10^6)*7*(10^-15)*(2^x)};
\addplot[color=orange, domain=14:30]{(1.09733*10^7)*7*(10^-15)*(2^x)};
\addplot[color=green, domain=14:24]{(5.34698*10^5)*((7*10^-15)*(2^x)+7/3*(10^-18)*(2^x)^2)};
\addplot[color=blue, domain=14:21]{(5.51075*10^6)*((7*10^-15)*(2^x)+7/3*(10^-18)*(2^x)^2)};
\addplot[color=purple, domain=14:21]{(1.09733*10^7)*((7*10^-15)*(2^x)+7/3*(10^-18)*(2^x)^2)};
\addplot[color=red,mark=diamond] coordinates {(23.2635,0) (23.2635,20) (23.2635,40) (23.2635,50)};

\addplot[mark=square] coordinates{ (16.66667, 0) (16.66667,20) (16.66667,40)  (16.66667, 50)};
\addplot[color=black, style=dotted, domain=0:30]{4};
\addplot[color=black, style=dashed, domain=0:30]{30};

\end{axis} 
\end{tikzpicture}
\caption{$C_H=\$7\times10^{-15}$, $C_{mem}=\$2.33\times10^{-18}$}
\label{fig:mhf}
\end{figure}

Specifically, the thresholds for memory hard functions fall below $\tau=23.2635$, and so rational adversaries choose not to crack all passwords, while server authentication still requires less than $1$ second.
Similarly, in Figure~\ref{fig:mhf2}, we show the effects of memory hard functions for general ratios $v/k$.

\begin{figure}[htb]
\centering
\begin{tikzpicture}[scale=0.9] 
\begin{axis}[title style={align=center},
	 title={Effects of Memory Hard Functions},
   xlabel={$\log_2(\tau)$},
   ylabel={$\%$ cracked},
	 xmin={18},
	 xmax={35},
	 ymin={0},
	 ymax={100},
   ylabel shift = -3pt,
   grid=major,
	 cycle list = {{blue, mark=none},  {green, mark=none}},
   legend style = {font=\tiny, at={(.95,.95)}, anchor=north east},
	 legend entries = {Yahoo! MHF, Yahoo!, $\max \#$ SHA256 hashes in 1sec $(10^7)$}
  ] 
%solve((x^0.871)/0.01413 - x/(1-0.871) = 4 / (((2^19)*7*10^-15)+(2.33*10^-18)*(2^19)^2), x)
%sum(0.01413/x^0.871,x,1,8)
\addplot coordinates{(18.58,100) (18.59,76.028) (18.6, 74.6487) (18.667, 70.6515) (19, 60.8578) (20, 43.885) (21, 32.4385)
									(22, 23.8261) (23, 17.1290) (24, 11.8327) (25, 7.6158) (26, 4.2857) (27, 1.413)};
%solve((x^0.871)/0.01413 - x/(1-0.871) = 4 / ((2^20)*7*10^-15), x)
\addplot coordinates{(25.63, 100) (25.64, 75.8317) (25.65,75.0902) (26, 66.8551) (27, 55.2655) (28, 47.0484) (29, 40.3712) (30, 34.7171)
									(31, 29.8337) (32, 25.5673) (33, 21.81125) (34, 18.4916) (35, 15.5406)};
\addplot[color=red,mark=diamond] coordinates {(23.2635,0) (23.2635,33) (23.2635,67) (23.2635,100)};
\end{axis} 
\end{tikzpicture}
\caption{$v=\$4$, $C_H=\$7\times10^{-15}$, $C_{mem}=\$2.33\times10^{-18}$}
\label{fig:mhf2}
\end{figure}
